# Supplementary material for: An unbiased approach to compressed sensing
Source: arXiv:1806.05283 source file (2021-04-05)
Supplement: Supplementary file 1 [file suppl_mat_unbiased_nobeta.tex]

\newpage

\begin{center}
{\Large \bf Proofs and further results\par}
\vspace*{24pt}
\end{center}

\section{Uniqueness of minimizers and stationary points with the desired property}\label{sec:unique}
We now turn to the heart of the matter, namely uniqueness of sparse minimizers of $\K_{reg}$, more precisely minimizers in a given $k$-sparse set $P_k$.
As noted in the introduction, this is not possible without imposing additional conditions on $A$ as well as $b$. In this section we provide such a condition and in the coming ones we show what it entails in practice for the sparsity (and $k$-sparsity) problem.

We recall that the \emph{subdifferential} of a function \( g  \) is the set-valued operator \( \partial g \) defined by \[ \partial g (x) = \{ u \, : \, g(y) \ge g(x) + \langle u , y -x \rangle \ \forall \, y  \}. \] The elements of \( \partial g (x)  \) are the \emph{subgradients} of \(g\) at \( x\).

We say that a point $x$ is a stationary point of $g$ if $0\in \partial g(x)$. For the case when $g$ is a sum of a convex function $g_c$ and a differentiable function $g_d$, it is easy to see that $x$ is a stationary point if and only if $-\nabla g_d(x)\in \partial g_c(x)$ where $\partial g_c(x)$ denotes the usual subdifferential. Set \begin{equation}\label{gdef}\G(x)=\frac{1}{2}\Q_2(f)(x)+\frac{1}{2}\fro{x},\end{equation} i.e. $2\G$ the l.s.c. convex envelope of $f(x)+\fro{x}$.
We have
\begin{equation}\label{fr3}\K_{reg}(x)=2\G(x)-\fro{x}+\fro{Ax-b}\end{equation}
which upon differentiation yields that $x'$ is a stationary point of $\K_{reg}$ if and only if
\begin{equation}\label{sp}(I-A^* A)x' + A^* b\in\partial \G(x').\end{equation}
Given any $x$, we therefore associate with it a new point $z$ via
\begin{equation}\label{y}
z=(I-A^* A)x + A^* b.
\end{equation}
The importance of $z$ is due to the following simple observation.

\begin{proposition}\label{thm:statpoint}
Let $x'$ and $x''$ be distinct stationary points of $\K_{reg}$ such that $x''-x'\in P_k$. Then
\begin{equation}\label{ineq}\re\scal{z''-z',x''-x'}\leq \delta_k^-\fro{x''-x'}.\end{equation}
\end{proposition}

The above proposition will mainly be used backwards, i.e.~we will show that \eqref{ineq} does not hold and thereby conclude that $x''-x'\not\in P_k$.

\begin{proof}
We have $$z''-z'=( I-A^* A)x''+A^*b-( I-A^* A)x'-A^*b=(I-A^* A)(x''-x'),$$
so taking the scalar product with $x''-x'$ gives $$\re\scal{z''-z',x''-x'}=\fro{x''-x'}-\fro{A(x''-x')}\leq \delta_k^-\fro{x''-x'},$$ as desired. Note that it is not necessary to take the real part, but we leave it since scalar products in general can be complex numbers.
\end{proof}

As we shall see, the point $z'$ has a decisive influence on the coming sections. To begin with, it has the following interesting property.

\begin{proposition}
A point $x'$ is a stationary point of $\K_{reg}$ if and only if it solves the convex problem $$x'\in\argmin_x \Q_2(f)(x)+\fro{x-z'}.$$
\end{proposition}
Note the absence of $A$ in the above formula, which in particular implies that $\Q_2(f)(x)+\fro{x-z'}$ is the convex envelope of $f(x)+\fro{x-z'}$.
\begin{proof}
As noted in \eqref{sp}, $x'$ is a stationary point of $\K_{reg}$ if and only if $z'\in\partial\G(x')$. By the same token, $x'$ is a stationary point of $$\Q_2(f)(x)+\fro{x-z'}=2\G(x)-2\scal{x,z'}+\fro{z'}$$ if and only if $z'\in\partial\G(x')$, and since the functional is convex (and clearly has a well defined minimum) the stationary points coincide with the set of minimizers.
\end{proof}

\section{The sparsity problem}\label{seccard}

We return to the sparsity problem, and consider $f(x)=\mu\card(x)$ where $\mu$ is a parameter and $\card (x)$ is the number of non-zero entries in the vector $x$. In this case we have,
\begin{equation}\label{l0000}\Q_2(\mu\card)(x)=\sum_{j=1}^n \mu-\para{\max\{\sqrt{\mu}-{ |x_j|},0\}}^2, \quad x\in\R^n.\end{equation}
To recapitulate, we want to minimize \eqref{q1}, i.e.~\begin{equation}\label{t57}\kfi(x)=\mu\card(x)+\fro{Ax-b}\end{equation} which we replace by \eqref{q1reg}, i.e. \begin{equation}\label{fr2}\kfir(x)=\Q_2(\mu\card)(x)+\fro{Ax-b}.\end{equation}

\subsection{Equality of minimizers for $\kfi$ and $\kfir$}

As noted by Aubert, Blanc-Feraud and Soubies (see Theorems 4.5 and 4.8 in \cite{soubies-etal-siims-2015}),
$\kfir$ has the same global minima and potentially fewer local minima than $\kfi$ if \begin{equation}\label{alpha}\|A\|_{\infty,col}=\sup_i \|a_i\|_2\leq 1,\end{equation} where $a_i$ denotes the columns of $A$. Below we (essentially) reproduce their statement in the terminology of this paper, and also include a proof for completeness.

\begin{theorem}\label{celok5}
If $\|A\|_{\infty,col}<1$, then any local minimizer of $\kfir$ is a local minimizer of $\kfi,$ and the (nonempty) set of global minimizers coincide. If merely $\|A\|_{\infty,col}=1$, then any connected component of global minima of $\kfir$ includes at least two global minima of $\kfi$.
\end{theorem}

\begin{proof}
We first establish that $\inf \kfi=\inf \kfir$. Since $\kfi\geq \kfir$ it suffices to show that $\inf \kfi\leq \inf \kfir$. Suppose not and let $x_0$ be a point such that $\kfir(x_0)<\inf \kfi$. Then there must be some index $j$ such that the corresponding value in $\Q_2(\mu\card)(x_0)$ is different from $\mu\card (x_{0,j})$, which (see \eqref{l0000}) implies that \begin{equation}\label{py1}0<|x_{0,j}|<\sqrt\mu.\end{equation} But then \begin{equation}\label{py}\partial_{x_{0,j}}^2\kfir(x_0)=-2+2\|a_j\|_2^2\leq 0.\end{equation} It follows that we can redefine $x_{0,j}$ to equal either $0$ or $\sqrt{\mu}$, so that the resulting point $x_1$ satisfies $\kfir(x_1)\leq \kfi(x_0)$. We can now continue like this for another index $j$ such that \eqref{py1} holds (if it exists), and this process must terminate after finitely many steps $N$. Denoting the resulting point by $x_N$, we see that it satisfies $\kfi(x_N)=\kfir(x_N)<\inf \kfi$, a contradiction.

It is easy to see that $\kfi$ has global minimizers, and by the above argument these are also global minimizers for $\kfir$. Now let $x_0$ be a global minimizer of $\kfir$ but not for $\kfi$. As before we have that \eqref{py1} and \eqref{py} holds for some index $j$, and we clearly must have equality in the latter. If $\|A\|_{\infty,col}<1$ this is a contradiction, and hance we see that the global minimizers of $\kfi$ and $\kfir$ coincides. If merely $\|A\|_{\infty,col}=1$, then we can redefine $x_{0,j}$ to equal either $0$ or $\sqrt{\mu}$ without changing the value of $\kfir$, and as before this process eventually leads to a point $x_N$ which is also a global minimizer for $\kfi.$ By the construction, there are at least two such points.

It remains to prove the statement about local minimizers. If $x_0$ is a local minimizer of $\kfir$ and $\|A\|_{\infty,col}<1$, we immediately get a contradiction from \eqref{py} unless $\kfi(x_0)=\kfir(x_0)$. In view of $\kfi\geq \kfir$, this establishes the claim.
\end{proof}

\subsection{On the uniqueness of sparse stationary points}\label{erai}
%Given subset $S\subset\{1,\ldots,n\}$ we define $A_S$ to be the matrix whose columns are $a_j$ for $j\in S$ and $0$ else.
Next we take a closer look at the structure of the stationary points. Given $N$ such that $\delta_{N}^-<1$, we will show that under certain assumptions the difference between two stationary points always has at least $N$ elements.
Hence if we find a stationary point with less than $N/2$ elements then we can be sure that this is the sparsest one. The main theorem reads as follows:

\begin{theorem}\label{thm:statpoint:vec}
Let $x'$ be a stationary point of $\kfir$, let $z'$ be given by \eqref{y}, and assume that
\begin{equation}\label{e4}|z_i'|\not\in\left[{(1-\delta_N^-)}{\sqrt{\mu}},\frac{{\sqrt{\mu}}}{1-\delta_N^-}\right]\end{equation} for all $i\in\{1,\ldots,n\}$.
If $x''$ is another stationary point of $\kfir$ then $\card(x''-x') > N$.
\end{theorem}

%With $N=2k$ we get the following corollary.

%\begin{corollary}\label{cor:statpoint:vec}
%Let $x'$ be a stationary point of $\kfir$, let $z'$ be given by \eqref{y}, and assume that
%\begin{equation}\label{e4c}|z_i'|\not\in\left[{\beta_{2k}^2}{\sqrt{\mu}},\frac{1}{\beta_{2k}^2}{\sqrt{\mu}}\right].\end{equation}
%If $x''$ is another stationary point of $\kfir$ then $\card(x'') > k$.
%\end{corollary}

Note that we allow $\delta_N^-<0$ in the above theorem, in which case the condition on $z'$ is automatically satisfied. The proof depends on a sequence of lemmas, and is given at the end of the section. Clearly, we will rely on Proposition \ref{thm:statpoint}, which requires an investigation of the functional $\G$ \eqref{gdef} and in particular its sub-differential. Introducing the function $g$ as
\begin{equation}
g(x) =
\begin{cases}
\frac{\mu + {x^2}}{2} & |x| \geq {\sqrt{\mu}} \\
\sqrt{\mu}|x| & 0 \leq |x| \leq {\sqrt{\mu}}
\end{cases}.
\label{eq:gdef}
\end{equation}
we get \begin{equation}\label{Gg}
\G(x)=\sum_{j=1}^n g(x_j).\end{equation}
Its sub-differential is given by
\begin{equation}
\partial g(x) =
\begin{cases}
\{ x\} & |x| \geq {\sqrt{\mu}} \\
\{\sqrt{\mu}\frac{x}{|x|}\} & 0 < |x| \leq {\sqrt{\mu}} \\
\sqrt{\mu}~\D & x = 0
\end{cases}
\label{eq:vectorsubgrad}
\end{equation} where $\D$ is the closed unit disc in $\C$ or, if working over $\R$, $\D=[-1,1]$. In the remainder we suppose for concreteness that we work over $\C$ (but show the real case in pictures).
Note that the sub-differential consists of a single point for each $x \neq 0$.
Figure~\ref{fig:gfunk} illustrates $g$ and its sub-differential.
\begin{figure}[htb]
\begin{center}
\includegraphics[width=40mm]{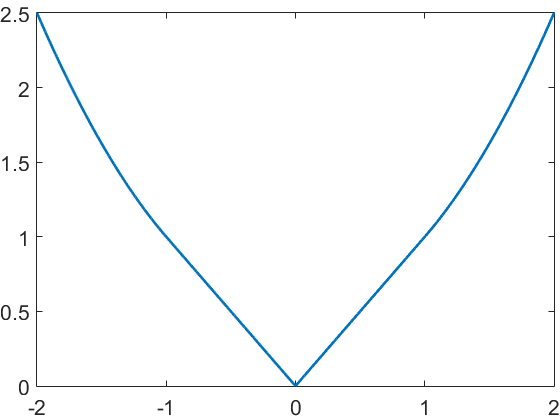}
\includegraphics[width=40mm]{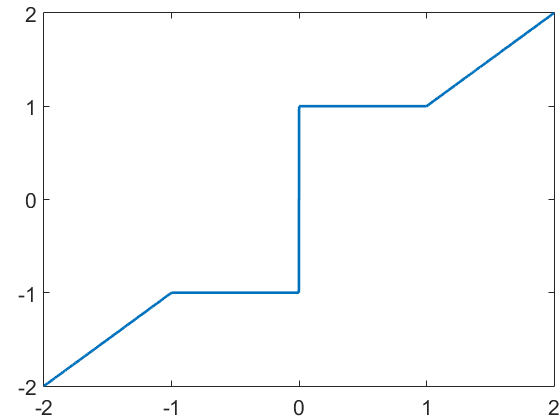}
\end{center}
\caption{The function $g(x)$ (left) and its sub-differential $\partial g(x)$ (right). Note that the sub-differential contains a unique element everywhere except at $x=0$.}
\label{fig:gfunk}
\end{figure}

%Our goal is now to find constraints that assure that this system of equations have only one solution. Before getting into the details we outline the overall idea.
%For simplicity consider two differentiable strictly convex functions $\tilde{h}$ and $\tilde{g}$.
%Their sum is minimized by the stationary point $x_s$ fulfilling $- \nabla \tilde{h}(x_s) = \nabla \tilde{g}(x_s)$.
%Since $\tilde{g}$ is strictly convex its directional derivative $\nabla \tilde{g} (x_s + t \v)^T \v$ is increasing for all $\v \neq 0$.
%Similarly $-\nabla \tilde{h} (x_s + t \v)^T \v$ is decreasing for all $\v\neq 0$ since $-\tilde{h}$ is strictly concave. Therefore $-\nabla \tilde{h} (x_s + t \v)^T \v < \nabla \tilde{g} (x_s + t \v)^T \v$ which means that $x_s$ is the only stationary point.
%In what follows we will estimate the growth of the directional derivatives of the functions involved in \eqref{eq:vectorobj} in order to show a similar contradiction.
%For the function $h$ we do not have convexity, however due to \eqref{eq:vectorRIP} we shall see that it behaves essentially like a convex function for sparse vectors $x$. Additionally we have to consider the non-convex perturbation $-\delta \|x\|^2$. Therefore we need somewhat sharper estimates than just growth of the directional derivatives of $g$.

The following two results establish a bound on the sub-gradients of $\G$.  We begin with some one-dimensional estimates of $g$.
%Due to convexity of $g$ it is clear that at any point $x$ these are growing in all directions $\v$.
%However, in order to guarantee uniqueness of a sparse stationary point we need to show that they grow faster than $2\delta \|\v\|^2$.
%Loosely speaking we will show that provided that the vector $\frac{1}{2}z$, where $z \in \partial g (x)$ is the sub-gradient, has elements that are not too close to the thresholds $\pm \sqrt{\mu}$ this will be true.

\begin{lemma}\label{lemma:bnd1}
Assume that $z_0 \in \partial g(x_0)$ and $\delta_N^->0$.
If
\begin{equation}
\left|
z_0
\right| > \frac{\sqrt{\mu}}{1-\delta_N^-}
\label{eq:subgradbnd1}
\end{equation}
then for any $x_1,~z_1$ with $z_1\in \partial g(x_1)$ and $x_1\neq x_0$, we have
\begin{equation}\label{fd}
\re(z_1 -z_0)\overline{(x_1-x_0)} > \delta_N^- |x_1-x_0|^2 .
\end{equation}
\end{lemma}
\begin{proof}
By rotational symmetry (i.e. $\partial g(e^{i\phi}x)= e^{i\phi} \partial g(x)$), it is no restriction to assume that $z_0>0$. By $\frac{1}{1-\delta_N^-}> 1$ and \eqref{eq:subgradbnd1}, we see that $z_0>\sqrt{\mu}$, and hence the identity $z_0\in\partial g(x_0)$ and \eqref{eq:vectorsubgrad} together imply that $z_0=x_0$ and in particular that $x_0\in\R$ and
\begin{equation}
\label{onion}x_0>\frac{\sqrt{\mu}}{1-\delta_N^-}.
\end{equation}
To prove the result we now minimize the quotient
$\frac{\re(z_1 -z_0)\overline{(x_1-x_0)}}{ |x_1-x_0|^2}$ and show that it is larger than $\delta_N^-$.
There are three cases to consider; $|x_1|=0$, $0<|x_1|<\sqrt{\mu}$ and $|x_1|\geq \sqrt{\mu}$. The latter case is easy since then $z_1-z_0=x_1-x_0$ and $\delta_N^- < 1$, which yields the desired conclusion.

For the two other cases we first show that $z_1$ and $x_0$ can be assumed to be real.
If $x_1=0$ then the optimization of the above quotient is equivalent to minimization of $-\re(z_1)$ over $z_1 \in \sqrt{\mu}\D$, since $x_0=z_0$ is real and positive, which is clearly minimized in $z_1 = \sqrt{\mu}$.
For the middle case, $z_1$ and $x_1$ have the same angle with $\R$, and $|x_1|<|z_1|<z_0$. We first hold the radii fixed and only consider the angle as an argument. Recall $z_0=x_0$ and set $R=|z_1|/|x_1|$. Then we have 
 \[ \begin{split} \frac{\re(z_1 -z_0)\overline{(x_1-x_0)}}{ |x_1-x_0|^2} & =\frac{R|x_1|^2-2R\re x_1 \overline{x_0}+|x_0|^2}{ |x_1-x_0|^2} \\ & = \frac{R(|x_1|^2-2\re x_1 \overline{x_0}+|x_0|^2) - R |x_0|^2 + |x_0|^2}{|x_1-x_0|^2}  \end{split}  \] that equals \begin{equation}\label{gt}R- \frac{R-1}{|x_1-x_0|^2} |x_0|^2 \end{equation}
which shows that the quotient is minimized when $x_1$ is real and $0<x_1<\sqrt{\mu}$ (which then automatically applies to $z_1$ as well).

Summarizing the above we may thus assume that $x_1$ and $z_1$ are real and non-negative and $0\leq x_1<\sqrt{\mu}$. This simplifies the quotient \eqref{gt} to $\frac{x_0-z_1}{ x_0-x_1}$. We now hold $x_1,~z_1$ fixed and consider $x_0$ as the variable. Since $z_1\geq x_1$, it is easy to see that this is minimized for $x_0$ as small as possible, i.e. $x_0=\frac{\sqrt{\mu}}{1-\delta_N^-}$. With this at hand, the minimum of $\frac{|z_1-\frac{\sqrt{\mu}}{1-\delta_N^-}|}{ |x_1-\frac{\sqrt{\mu}}{1-\delta_N^-}|}$ is clearly attained at $x_1=0$ and $z_1=\sqrt{\mu}$. Summing up, we have that
$$\frac{\re(z_1 -z_0)\overline{(x_1-x_0)}}{ |x_1-x_0|^2}>\frac{|z_1-\frac{\sqrt{\mu}}{1-\delta_N^-}|}{ |x_1-\frac{\sqrt{\mu}}{1-\delta_N^-}|}\geq \frac{|\sqrt{\mu}-\frac{\sqrt{\mu}}{1-\delta_N^-}|}{ |\frac{\sqrt{\mu}}{1-\delta_N^-}|}=\delta_N^-.$$
\end{proof}

\begin{lemma}\label{lemma:bnd2}

Assume that $z_0 \in \partial g(x_0)$ and $\delta_N^->0$.
If
\begin{equation}
\left|
z_0
\right| < {(1-\delta_N^-)}{\sqrt{\mu}}
\label{eq:subgradbnd2}
\end{equation}
then for any $x_1,~z_1$ with $z_1\in \partial g(x_1)$, $x_1\neq x_0$, we have
\begin{equation}\label{fd1}
\re(z_1 -z_0)\overline{(x_1-x_0)} > \delta_N^- |x_1-x_0|^2.
\end{equation}\end{lemma}
\begin{proof}
The proof is similar to the previous lemma. We first note that $x_0=0$, $x_1\neq 0$ and that $z_0$ may be assumed to be in $(0,\sqrt{\mu}]$. For a fixed radius $R = \frac{|z_1|}{|x_1|}$ the quotient \[\frac{\re(z_1 -z_0)\overline{(x_1-x_0)}}{ |x_1-x_0|^2}=\frac{\re(z_1 -z_0)\overline{x_1}}{ |x_1|^2} = R- z_0\frac{\re  x_1}{|x_1|^2} \] is smallest when both $x_1$ and $z_1$ are real valued and positive.
Since $x_1\neq 0$ we have $z_1 = \max(x_1,\sqrt{\mu})$.
Clearly $z_0={(1-\delta_N^-)}{\sqrt{\mu}}$ gives a minimum value for any positive choice of $x_1,z_1$, because \( |z_0 \re (x_1) / |x_1|^2 | < {(1-\delta_N^-)}{\sqrt{\mu}} | \re (x_1) / |x_1|^2 |   \).
This reduces the problem to finding the minimum of $$x_1 \mapsto\frac{\max(x_1,\sqrt{\mu}) -{(1-\delta_N^-)}{\sqrt{\mu}}}{ x_1}$$ which by basic calculus equals $\delta_N^-,$ as desired.
\end{proof}

We are now ready to prove Theorem \ref{thm:statpoint:vec}.

\begin{proof}[Proof of Theorem \ref{thm:statpoint:vec}]
By Proposition \ref{thm:statpoint} it suffices to verify \begin{equation}\label{g}
\re\skal{z''-z',x''-x'} > \delta_N^- \|x''-x'\|_2^2,\quad x''\neq x'.
\end{equation} The claim will follow by contradiction.
Suppose first that $\delta_N^->0$. Since $\partial \G(x)=\sum_{j=1}^n \partial g(x_j)$, Lemmas \ref{lemma:bnd1} and \ref{lemma:bnd2} imply that
$$\re(z''_i-z'_i) \overline{(x_i''-x_i')} > \delta_N^- |x_i''-x_i'|^2,
$$
for all $i$ with $x_i''-x_i' \neq 0$. Since $x_i''-x_i'=0$ gives $(z''_i-z'_i)\overline{(x_i''-x'_i)}=0$
summing over $i$ gives the result.

Suppose now that $\delta_N^->1$. By \eqref{g} it suffices to prove that $\re\skal{z''-z',x''-x'}\geq 0$ for all $x''\neq x'$. Fix $i$ in $\{1,\ldots,n\}$. By rotational symmetry it is easy to see that we can assume that $x'_i,z'_i\geq 0$. Moreover, for fixed values of $|z_i''|$ and $|x''_i|$ (but variable complex phase) it is easy to see that $\re (z_i''-z')(x_i''-x_i')$ achieves min when these are also real, i.e. we can assume that $x''_i,z''_i\in\R$. Since the graph of $\partial g$ is non-decreasing it follows that $(z_i''-z')(x_i''-x_i') \geq 0$ for all $i$, as desired.

It remains to consider the case when $\delta_N^-=1$, and as above we reach a contradiction if we prove that $\re\skal{z''-z',x''-x'}> 0$. Again we can assume that $x'_i,z'_i\geq 0$ and that $x''_i,z''_i\in\R$. Then \eqref{e4} implies that $z_i'\neq \sqrt{\mu}$ for all $1\leq i \leq n$, which via $z'_i\in \partial g(x'_i)$ also implies that $x_i'\not\in (0,\sqrt{\mu}]$. If $x''\neq x'$ we must have $x''_i\neq x_i$ for some $i$. Using that $z_i''\in \partial g$, examination of \eqref{eq:vectorsubgrad} yields that also $z_i''\neq z_i'$.
With this at hand we see that the left hand side of \eqref{g} is strictly positive, whereas the right equals 0, which again is a contradiction.

\end{proof}

\iffalse
For later use in [..], we record that we have shown the following result. \begin{corollary}\label{corbor}
Let $z'$ satisfy $z'\in\partial \G(x')$ and
\begin{equation}\label{e4t}|z_i'|\not\in\left[{\lambda^2}{\sqrt{\mu}},\frac{1}{\lambda^2}{\sqrt{\mu}}\right].\end{equation}
If $z''\in\partial \G(x'')$, then $\re\scal{z''-z',x''-x'}>(1-\lambda^2)\|x''-x'\|_2^2$.
\end{corollary}
\fi

\subsection{Conditions on global minimality}\label{erai1}

\begin{theorem}\label{thm:globalpoint2}
Let $A$ satisfy $\|A\|_{\infty,col}\leq 1$, let $x'$ be a stationary point of $\kfir$ and let $z'$ be given by \eqref{y}. Assume that
\begin{equation}\label{cond3}|z_i'|\not\in\left[{(1-\delta_N^-)}{\sqrt{\mu}},\frac{1}{1-\delta_N^-}{\sqrt{\mu}}\right],\quad 1\leq i\leq n.\end{equation}
If \begin{equation}\label{cond2}2\mu\card(x') +\fro{Ax'-b}< \mu N+\mu,\end{equation} then $x'$ is the unique global minimum of $\kfi$ and $\kfir$.
\end{theorem}

Obviously, it is desirable to pick $N$ as large as possible, which is limited by \eqref{cond3} and the fact that $\delta_N^-$ increases with $N$. Also note that $\delta_N^-\geq 0$ since $1-\delta_1^-\leq \sup_i\{\|a_i\|_2^2\}=\|A\|_{\infty,col}^2\leq 1$.

\begin{proof}
Set $k=\card(x')$ and assume that $x'$ is not the unique global minimizer of $\kfir$.
By Theorem \ref{celok5}, there exists a global minima $x''\neq x'$ for both $\kfir$ and $\kfi$, which hence is a stationary point of $\kfir$. Theorem \ref{thm:statpoint:vec} then shows that $\card (x'')\geq N-k+1$. It follows that
$$\kfir(x'')-\kfir(x')\geq \kfi(x'')-\kfi(x')\geq \mu(N-k+1)-(\mu k +\fro{Ax'-b})>0$$
by \eqref{cond2}, $\kfi(x'')=\kfir(x'')$ and $\kfi(x')\geq\kfir(x')$. This is a contradiction, and hence $x'$ must be the unique global minimizer of $\kfir$. By Theorem \ref{celok5} it then follows that $x'$ is also unique minimizer of $\kfi$.
\end{proof}

\subsection{Noisy data.}
In this final subsection we return to the compressed sensing problem of retrieving a sparse vector $x_0$ given corrupted measurements $b=Ax_0+\ep$, where $\ep$ is noise and $x_0$ is sparse. More precisely we set $S=\supp x_0$ where we assume that $\#S=k$ is much smaller than $m$ -- the amount of rows in $A$ (i.e. number of measurements). We let $x_{0,j}$ denote the elements of the vector $x_0$. Let $A_S$ denote the matrix obtained from $A$ by setting columns outside of $S$ to $0$, and let $x_S$ denote the least squares solution to $A_S x_S=b$. Note that this is the so called ``oracle solution'' discussed in the introduction, which can also be written $x_S=(A_S^*A_S)^\dagger A_S^*b$ where $(A_S^*A_S)^\dagger$ denotes the Moore-Penrose inverse. The below proposition shows that the oracle solution is under mild assumptions a local minimizer of $\K_{reg}$, which we denote by $x'$ for notational consistency.

\begin{proposition}\label{p1}
Let $A$ satisfy $\|A\|_{\infty,col}\leq 1$. If $\|\ep\|_2< {\sqrt{\mu}}$ and $$|x_{0,j}|>\sqrt{\mu}+\frac{\|\ep\|_2}{\sqrt{1-\delta_k^-}}$$ for all $j\in S$ then the oracle solution $x'=x_S$ is a strict local minimum to $\kfir$ with $\supp (x')=\supp (x_0)$. We also have $|x_{j}'|>\sqrt{\mu},~ j\in S,$ $\|Ax'-b\|_2\leq \|\epsilon\|_2$, and $$\|x'-x_0\|_2\leq \frac{\|\ep\|_2}{\sqrt{1-\delta_k^-}}.$$
\end{proposition}
%do we need to prove this or showing stationary point is enough??????????
\begin{proof}
Consider the equation $A_Sx=Ax_0+\ep$ and note that $Ax_0=A_Sx_0$. The least squares solution is obtained by applying $(A_S^*A_S)^\dagger A_S^*$ which gives the solution $$x'=x_0+(A_S^*A_S)^\dagger A_S^*\ep=x_0+\eta,$$ where we set $(A_S^*A_S)^\dagger A_S^*\ep=\eta$. By construction of the Moore-Penrose inverse, $\supp \eta\subset S$, and hence $$A\eta=A_S\eta=P_{\text{Ran} A_S}\ep,$$ where $P_{\text{Ran} A_S}$ denotes the orthogonal projection onto the range of $A_S.$ In particular, $$\|\eta \|_2\leq\frac{\|A_S\eta\|_2}{\sqrt{1-\delta_k^-}}=\frac{\|P_{\text{Ran} A_S}\ep\|_2}{\sqrt{1-\delta_k^-}}\leq \frac{\|\ep\|_2}{\sqrt{1-\delta_k^-}},$$
which establishes the final inequality in the proposition. Also $\|\eta\|_{\infty}\leq \|\eta\|_{2}$ which implies \begin{equation}\label{sofg}|x_{j}'|\geq |x_{0,j}|-|\eta_j|>\sqrt{\mu}+\frac{\|\ep\|_2}{\sqrt{1-\delta_k^-}}-\frac{\|\ep\|_2}{\sqrt{1-\delta_k^-}}=\sqrt{\mu},\quad j\in S.\end{equation} This also gives $\supp x'=\supp x_0$ since by construction we clearly have \[\supp x' \subset \supp x_0\cup\supp \eta \subset S.\]

We now consider $Ax'-b$, which equals \begin{equation}\label{sof}\begin{aligned}&=A_Sx'-b\\&=A_Sx_0+A_S(A_S^*A_S)^\dagger A_S^*\ep-(A_Sx_0+\ep)\\&=(P_{\text{Ran} A_S}-I)\ep\\&=-P_{(\text{Ran} A_{S})^{\perp}}\ep\end{aligned}\end{equation}
and hence $\|Ax'-b\|_2\leq \|\epsilon\|_2$.

It remains to prove that $x'$ is a local minimum of $\kfir=\Q_2(\mu\card)+\fro{Ax-b}$. To this end, consider $\kfir(x'+v)$. Since $|x_{j}'|>\sqrt{\mu}$ for $j\in S$, the term $\Q_2(\mu\card)$ is flat for the corresponding indices of $v$. We get \begin{equation}\label{rd}\kfi(x'+v)=\sum_{j\in S^c}\left(2\sqrt{\mu} |v_j|-v_j^2\right)+2\scal{v,A^*(Ax'-b)}+\|Av\|_2^2+\kfir(x').\end{equation} Since $x'$ solves the least squares problem posed initially, the vector $A_S^*(Ax'-b)=A_S^*(A_Sx'-b)$ must be 0. With this in mind \eqref{rd} then simplifies to \begin{equation}\label{rd1}2\left(\sum_{j\in S^c}\sqrt{\mu} |v_j|+v_j\scal{a_j,Ax'-b}\right)-\sum_{j\in S^c}v_j^2+\|Av\|_2^2+\kfir(x').\end{equation} By the Cauchy-Schwartz inequality and \eqref{sof} we have $$|\scal{a_j,Ax'-b}|\leq \|a_j\|_2\|\ep\|_2< \|A\|_{\infty,col} {\sqrt{\mu}}\leq\sqrt{\mu}.$$ It follows that the term $\sum_{j\in S^c}\sqrt{\mu} |v_j|+v_j\scal{a_j,Ax'-b}$ in \eqref{rd1} can be estimated from below as follows: \[  > \sum_{j \in S^c}  |v_j|( \underbrace{\sqrt{\mu} + \min\{ 0,\text{sign}(v_j) \langle a_j, A x' - b \rangle\}}_{:= \alpha_j}   ) \ge \rho\sqrt{\sum_{j\in S^c}v_j^2}     \]for some $\rho>0$, where \( \alpha_j > 0  \) for all \(j\) and we used the equivalence between \( \ell^1 \) and \( \ell^2  \) norms. Hence $$2\left(\sum_{j\in S^c}\sqrt{\mu} |v_j|+v_j\scal{a_j,Ax'-b}\right)-\sum_{j\in S^c}v_j^2>0$$ for $v$ in a neighborhood of 0, as long as $\sum_{j\in S^c}v_j^2\neq 0$. To have $\kfir(x'+v)\leq\kfir(x')$ we thus need $\supp v\subset S$, as seen from \eqref{rd1} (and this because both summations in \eqref{rd1} are over \( S^c \), but if $\supp v\subset S$ then \( v_j = 0  \) for all \( j \in S^c \)). But then \eqref{rd1} reduces to $\|Av\|_2^2+\kfir(x')$, and since ${\delta_k^-}<1$ it follows that $\|Av\|_2^2>0$ unless $v=0$. In other words, $x'$ is a strict local minimizer.
\end{proof}

%By the above proof, an explicit formula for $x_1$ is
%\begin{equation}\label{ko}x_1=x_0+(A_S^*A_S)^\dagger A_S^*\ep.\end{equation}

In the above proposition, there is nothing said as to whether $x'$ is a global minimum or not. To get further, let $z'$ correspond to $x'$ via \eqref{y}. We need conditions such that \eqref{cond3} holds for $z'$, i.e.
\begin{equation}\label{cond31}|z_{i}'|\not\in\left[{(1-\delta_N^-)}{\sqrt{\mu}},\frac{{\sqrt{\mu}}}{1-\delta_N^-}\right].\end{equation}
We remind the reader that $N$ is a number which preferably is a bit larger than $2k$, where $k$ is the cardinality of $x_0$.

\begin{proposition}\label{p2}
Let $A$ satisfy $\|A\|_{\infty,col}\leq 1$. If $\|\ep\|_2< {(1-\delta_N^-)\sqrt{\mu}}$ and \begin{equation}\label{po7}|x_{0,j}|>\frac{\sqrt{\mu}}{1-\delta_N^-}+\frac{(1-\delta_N^-)\sqrt{\mu}}{\sqrt{1-\delta_k^-}}, \quad j\in \supp x_0,\end{equation}
then \eqref{cond31} holds.
\end{proposition}
\begin{proof}
Using \eqref{sof} we get
\begin{align}\label{tg}z'=( I-A^* A)x' + A^* b =  x'-A^*(Ax'-b)= x'+A^*P_{(\text{Ran} A_{S})^{\perp}}\ep.\end{align}
Since $A^*P_{(\text{Ran} A_{S})^{\perp}}$ is 0 on rows with index $j\in S$ (being a scalar product of a vector in $\text{Ran} A_{S}$ and another in its orthogonal complement), we see that $z_{j}'= x_{j}'$ for such $j$. Combining this with the final estimate of Proposition \ref{p1}, we see that  \begin{equation*}\label{po9}|z_{j}'|>\frac{1}{1-\delta_N^-}{\sqrt{\mu}}, \quad j\in S\end{equation*} holds whenever \begin{equation}\label{po6}|x_{0,j}|>\frac{\sqrt{\mu}}{1-\delta_N^-}+\frac{\|\ep\|_2}{\sqrt{1-\delta_k^-}}, \quad j\in S,\end{equation} which is true by the assumptions. For the remaining $z_{j}'$, (i.e. $j\in S^c$), we have $x_{j}'=0$ so \begin{equation}\label{o0}\begin{aligned}&|z_j'|=|(A^*P_{(\text{Ran} A_{S})^{\perp}}\ep)_j|=|\scal{P_{(\text{Ran} A_{S})^{\perp}}\ep,a_j}|\leq \\&\|A\|_{\infty,col}\|\ep\|_2\leq \|\ep\|_2<{(1-\delta_N^-)}{\sqrt{\mu}},\end{aligned}\end{equation}
which establishes \eqref{cond31}.
\end{proof}

Putting all the results together and combining with simple estimates, we finally get

\begin{theorem}\label{thm:doctorgadget}
Suppose that $b=Ax_0+\ep$ where $A$ is an $m\times n$-matrix with $\|A\|_{\infty,col}\leq 1$ and set $\card (x_0)=k.$ Let $N\geq 2k$ and assume that
$\|\ep\|_2< {(1-\delta_N^-)\sqrt{\mu}}$ and $$|x_{0,j}|>\para{\frac{1}{1-\delta_N^-}+1}\sqrt{\mu},\quad j\in \supp x_0.$$ Then the oracle solution $x'=x_S$ is a unique global minimum to $\kfir$ as well as $\kfi$, with the property that $\supp x'=\supp x_0$, that $$\|x'-x_0\|_2\leq \frac{\|\ep\|_2}{\sqrt{1-\delta_k^-}},$$ and that $\card(x'')> N-k$ for any other stationary point $x''$ of $\kfir$.
\end{theorem}

\iffalse
A necessary condition for the above assumptions to hold, is that they hold with $\beta_{N}$ replaced by $\sigma_{N}$, in light of Proposition \ref{p0}.
\fi
\begin{proof}
All the statements follow by Theorem \ref{thm:statpoint:vec}, Theorem \ref{thm:globalpoint2} and Proposition \ref{p1}, so we just need to check that these apply. Note that $\sqrt{1-\delta_{N}^-}\leq \sqrt{1-\delta_k^-}\leq \|A\|_{\infty,col}\leq 1$ which will be used repeatedly.

We begin to verify that Proposition \ref{p1} applies, which is easy by noting that $\|\ep\|_2\leq (1-\delta_N^-)\sqrt{\mu}<2\sqrt{\mu}$ and $${\sqrt{\mu}}+\frac{\|\epsilon\|_2}{\sqrt{1-\delta_k^-}}\leq \frac{\sqrt{\mu}}{1-\delta_N^-}+\frac{(1-\delta_N^-)\sqrt{\mu}}{\sqrt{1-\delta_k^-}}\leq \frac{\sqrt{\mu}}{1-\delta_N^-}+{\sqrt{\mu}}<|x_{0,j}|.$$

Now, to verify that the two theorems apply we need to check the conditions \eqref{cond31}, which follow if we show that Proposition \ref{p2} applies. The estimate on $\|\ep\|_2$ is satisfied by assumption and the other follows by noting that $\frac{1-\delta_N^-}{\sqrt{1-\delta_k^-}}\leq 1.$ By this we already have verified Theorem \ref{thm:statpoint:vec} and the first condition of Theorem \ref{thm:globalpoint2}. To check  \eqref{cond2} note that $\|Ax'-b\|_2\leq \|\ep\|_2< (1-\delta_N^-)\sqrt{\mu}$ by Proposition \ref{p1}, so \eqref{cond2} holds if $2\mu k+(1-\delta_N^-)^2{\mu}\leq \mu N+\mu$, which is clearly the case since $N\geq 2k$.

\end{proof}

As usual, a simpler statement is found by setting $N=2k$, which gives the loosest conditions to verify, (see Corollary \ref{cor:doctorgadget}). The only difference in the conclusion concerns the cardinality of other local minima, since the estimate on $\|x'-x_0\|_2$ only depends on $\delta_k^-$.

\section{Known model order; the $k$-sparsity problem}\label{seccardfix}

Let $P_k=\{x:\card (x)\leq k\}$ where $x$ is a vector in $\C^n$ or $\R^n$. Set $f(x)=\iota_{P_k}(x)$ and note that the problem \begin{equation}\label{agt1}\argmin_{\card(x)\leq k}\|Ax-b\|_2\end{equation} is equivalent to finding the minimum of \begin{equation}\label{agt2}\ksi(x)=\iota_{P_k}(x)+\|Ax-b\|_2^2,\end{equation}
(where we put a subindex $k$ to distinguish from $\K$ in the previous section). Again, we will approach this problem by using
$$\ksir(x)=\Q_2(\iota_{P_k})(x)+\|Ax-b\|_2^2.$$
This is in some ways much simpler than the situation in the previous sections, for example all local minimizers of $\ksi$ are clearly in $P_k$.
On the other hand, $\Q_2(\iota_{P_k})$ turns out to be rather complicated. We recapitulate the essentials, which follows by adapting the computations in \cite{andersson-etal-ol-2017} (for matrices) to the vector setting. Define $\tilde x$ to be the vector $x$ resorted so that $(|\tilde x_j|)_{j=1}^d$ is a decreasing sequence. Then
%\begin{equation}\label{lust2}\S(\iota_{P_k})(y)= \sum_{j=k+1}^d -|\tilde y_j|^2\end{equation}
\begin{equation}\label{lust1}\Q_2(\iota_{P_k})(x)= \frac{1}{k_*}\para{\sum_{j>k-k_*}|\tilde{x}_j|}^2-\sum_{j>k-k_*}|\tilde x_j|^2\end{equation} where $k_*$ is the largest value of \(l \in \{1,\dots,k\} \) for which the non-increasing sequence
\begin{equation}\label{lust}s(l)=\left(\sum_{j>k-l}|\tilde x_j|\right)-l|\tilde x_{k+1-l}|\end{equation}
is non-negative (note that it clearly is non-negative for $l=1$); finding \( k_* \) has complexity (at worst) \( O(d^2) \). Although it is not very clear from the above expression, $\Q_2(\iota_{P_k})$ is known to be continuous (see e.g.~Proposition 3.2 in \cite{carlsson2018convex}), and this will be used without comment below. We first show that the global minima of $\ksir$ and $\ksi$ coincide.

\subsection{Equality of minimizers and $k$-feasibility}\label{Kfeas}

In order to provide a theorem similar to \ref{celok5}, we need a technical condition on the columns $a_1,\ldots,a_n$ of $A$. We say that $A$ is \textit{$k$-feasible} if $\|A\|_{\infty,col}\leq 1$ and for any subset of $n-k$ columns, we can pick two such that $\|a_i-a_j\|_2^2\leq 2$. We say that $A$ is \textit{strictly $k$-feasible} if the inequality is strict. This is very easy to satisfy, the following proposition lists conditions that imply $k$-feasibility in $\R$ and $\C$ respectively.
\begin{proposition}\label{mfisR}
If we work over $\R$, any $A$ with $\|A\|_{\infty,col}\leq 1$ and $n\geq m+k+2$ is $k-$feasible. If we add the condition that $\scal{a_i,a_j}\neq 0$ for all pairs, or that $\|A\|_{\infty,col}< 1$, then strict $k-$feasibility follows. The same follows over $\C$ if $n\geq 2m+k+2$. Another condition ensuring strict $k-$feasibility, which works in both $\R$ and $\C$, is that $\|A\|_{\infty,col}\leq 1$ and at least $nk$ of the values $\{\re\scal{a_i,a_j}\}_{i> j}$ are positive (repetitions allowed).
\end{proposition}
We remark that it is possible to choose $2m+1$ vectors in $\C^m$ such that $\|a_i-a_j\|_2^2> 2$, just consider a simplex in $\R^{2m}$ with equal sidelengths and all corners on the unit sphere. The condition that $n\geq 2m+k+2$ is a bit unfortunate, since it rules out the common situation $n=2m$. This is why we added the final part of the proposition.

\begin{proof}
If the chosen subset contain a zero vector, the conclusion is immediate, so we can assume that this is not the case. For any $m+2$ vectors $a_1,\ldots,a_{m+2}$ in $\R^m$, we can always pick two such that $\scal{a_i,a_j}\geq 0$, which follows from a simple induction argument: this is indeed clear in \( \mathbb{R} \); in \( \mathbb{R}^{m} \) take \( m+2 \) vectors \( v_i\) such that \( \langle v_i , v_j \rangle < 0  \) if \( i \ne j  \). If \(V\) is the orthogonal to \( v_{m+2}  \), the projections of \( v_1, \dots , v_{m+1} \) on \( V  \) have the same property, and \( V\) is an \((m-1)\)-dimensional vector space. By induction we would get the same conclusion for \( \mathbb{R}  \), which is a contradiction.

The first two conclusions regarding $\R^m$ follow immediately by this observation. Since $\C^m$ is isomorphic with $\R^{2m}$, the corresponding result for $\C$ follows. Finally, the elements above the diagonal in $(\scal{a_i,a_j})_{i,j=1}^n$ are $n(n-1)/2$ in number. When we consider a subset of columns of cardinality $n-k$, we remove a total of $(n-k)k+(k-1)k/2$ of these. Since $nk$ is a bigger number, we are certain that at least one positive value remain.
\end{proof}

To illustrate a concrete example, which sometimes appears in applications, we consider the concatenation of a discrete Fourier transform matrix and an identity matrix. To see what the above proposition entails in this case, suppose that $m=4M$ or $m=4M+1$. Each column of the Fourier matrix gives rise to at least $M$ positive values in its scalar products with the canonical basis coming from the identity matrix, so in total we have at least $mM$ positive off diagonal elements in the Fourier matrix. This gives the condition $2mk\leq mM$, i.e.~$K\leq m/8$, which is acceptable for relevant applications. We now develop some theory for $k$-feasible matrices, starting with the analog of Theorem \ref{celok5}.

\begin{theorem}\label{celok6}
Let $A$ be $k$-feasible. Then the global minimizers of $\ksir$ and $\ksi$ coincides, and all lie in $P_k$. If $A$ is strictly $k$ feasible, then any local minimizer of $\ksir$ lies in $P_k$ and is a minimizer of $\ksi$.
\end{theorem}

\begin{proof} We first treat global minimizers. Clearly all minimizers of $\ksi$ are in $P_k$. Since $\ksi\geq\ksir$ and they coincide on $P_k$, it suffices to show that a given global minimizer of $\ksir$ is in $P_k$. This is annoyingly difficult, it is even a problem to show that $\ksir$ has global minima. We begin by showing that large values of $x$ are not candidates for global minima if they are in the set $$U=\left\{x\neq 0:~\frac{\sum_{j=k+1}^n|\tilde x_j|}{\sum_{j=1}^k|\tilde x_j|}\geq\frac{1}{2k}\right\}.$$ We have $\Q_2(\iota_{P_k})(x)>0$ for all $x\in U$. One way to see this is by Corollary 4.4 in \cite{carlsson2018convex} (or Theorem 2.20 in \cite{carlsson2016convexification}), which states that there exists a direction $v$ such that $t\mapsto \Q_2(\iota_{P_k})(x+tv)>0$ has negative second derivative (since $\ksir(x)<\infty=\ksi(x)$), and this would imply that $\Q_2(\iota_{P_k})$ could take negative values, contradicting Proposition 3.2 in \cite{carlsson2018convex} (or Proposition 2.1 in \cite{carlsson2016convexification}). This can also be deduced by a more careful analysis of \eqref{lust1}, which we will perform below. Define \begin{equation}\label{olbia}\alpha =\inf\left\{\Q_2(\iota_{P_k})(x): ~x\in U,~\|x\|_2=1\right\}.\end{equation}
Since we are minimizing a continuous non-zero function over a compact set, $\alpha>0$. We now show that large values of $x\in U$ yield large values of $\Q_2(\iota_{P_k})(x)$. Let us write $s=s_x$ for \eqref{lust}, when there is a need to make the dependence on $x$ clear. The function $s$ is radially dependent, i.e.~$s_{tx}=t s_x$ for $t\in\R$, and hence $k_*$ is radially independent. Looking at the expression for $\Q_2(\iota_{P_k})$ we see that $$\Q_2(\iota_{P_k})(tx)=t^2\Q_2(\iota_{P_k})(x)\quad t\in \R.$$
Note that $\ksi(0)=\ksir(0)=\frac{1}{2}\|b\|_2^2$ so the global minimum is less than or equal to this. If $R$ is such that $\alpha R^2>\frac{1}{2}\|b\|_2^2$, it finally follows that no point $x\in U$ with $\|x\|_2>R$ can be less than $\frac{1}{2}\|b\|_2^2$.

We remark in passing that $x=0$ can not be a global minimizer of $\ksir$ unless $b$ is perpendicular to the range of $A$, in which case the theorem holds trivially. To see this, note that
$\Q_2(\iota_{P_k})(0)=0$ and $\Q_2(\iota_{P_k})\geq 0$, so if $x=0$ is the global minimum of $\ksir$ the gradient of $\frac{1}{2}\|Ax-b\|_2^2$ must necessarily be zero at $x=0$, i.e.~$A^*(-b)=0$.

Now let $G$ be the set of global minimizers for $\ksir$ restricted to $[-R,R]^n$. This set is clearly closed, non-void and bounded. Now let $G_n\subset G$ be the subset where $|\tilde x_n|$ attains its minimum over $G$, let $G_{n-1}\subset G_n$ be the subset where $|\tilde x_{n-1}|$ is minimized, and so on until we reach $G_{k+1}$, which still is closed, non-void and bounded. Suppose that $G_{k+1}\not\subset P_k$ and pick $x\in G_{k+1}\setminus P_k$. We now show that this is impossible. First of all, note that any two columns of $A$ and corresponding two elements in $x$ may (simultaneously) switch positions and sign, without affecting the problem, so it is no restriction to assume that $|\tilde x|=x$ (i.e. \( x_i \ge 0 \) and \( x_i \ge x_{i+1} \) for all \(i\)), which we now do.

If $x_{k+1}=R$ then this must also be the case for $x_1,\ldots,x_k$, and hence $\|x\|_2>R$ and $x\in U$, which is impossible by the earlier conclusions. Thus $x_{k+1}<R$.

Use $k$-feasibility of $A$ to pick two indices $j>i> k$ such that $\|a_i-a_j\|_2^2\leq 2$. Consider the function \begin{equation}\label{function}x(t)=x+t e_i-te_j.\end{equation} We shall show that this function stays in $G$ for small values of $t>0$, which contradicts the construction of $G_{k+1}$. Note that it stays in $[-R,R]^n$ for sure, due to $x_{k+1}<R$.

A complicating factor is the fact that we may fail to have $|\tilde x(t)|=x(t)$ for $t>0$, i.e.~this vector is not necessarily non-increasing as a function of its index. As long as $ x_{k}> x_{i}$, we can pick both $i,j>k$ such that $x(t)$ is non-increasing for small values of $t>0$. We consider this case first. All values of $s_{x(t)}(l)$ in \eqref{lust} are then unaltered by $t$, and hence small perturbations do not affect $k_*$. With this at hand, it follows that the first term in the expression \eqref{lust1} for $\Q_2(\iota_{P_k})(x(t))$ is unaffected by small changes in $t$, whereas the latter term is a quadratic polynomial starting with $-2t^2$. The quadratic term in the expression $\|Ax(t)-b\|_2^2$ on the other hand is $\|a_i-a_j\|_2^2t^2$. Using $\|A\|_{\infty,col}\leq 1$, it follows that \begin{equation}\label{po0}\frac{d^2}{dt^2}\ksir(x(t))=-4+2\|a_i-a_j\|_2^2\leq 0.\end{equation} Thus $\ksir(x(t))$ is linear in a neighborhood of 0, and since $x(0)\in G$ it must actually be a constant. It follows that $x(t)\in G$ for small values of $t>0$, which is a contradiction as we noted before.

It remains to consider the case when $x_{k}= x_{i}$. In this case we can make $x(t)$ non-increasing (of its index) for small (fixed) values of $t>0$, upon changing $i$ so that $x_i$ is the first value to equal $x_k$, but now $i\leq l$ and the independence of $k_*$ is less clear. Let $k_i$ be such that $i=k+1-k_i$. We will need the following observations about $s(l)$; If $x_{k+1-l}=x_{k+1-(l+1)}$ then $s(l)=s(l+1)$ so we always have \begin{equation}\label{inh}x_{k+1-k_*}<x_{k+1-(k_*+1)}=x_{k-k_*}.\end{equation} Since $x\not \in P_k$, we also have $s_x(1)>0$. Combined this gives $s_x(k_i)=s_x(1)>0$ and hence $k_*\geq k_i$. If we now consider $s_{x(t)}(l)$ as functions of $t$, the inequality $s_{x(t)}(k_i)>0$ is stable with respect to small perturbations. On the other hand, the values of $s_{x(t)}(l)$ for $l>k_i$ are unaffected by small values of $t$ (they cancel out in the sum of \eqref{lust}), and so we conclude that $k_*$ is unaffected by small values of $t$. It follows that both terms depending on $t$ in $ x(t)$ have indices beyond $k-k_*$, which precisely as before yields that \eqref{po0} holds, a contradiction.

To sum up, we have so far shown that any element $x\in G_{k+1}\setminus P_k$ necessarily satisfies $|\tilde x_{k+1}|<R$ and $|\tilde x_n|=0$. As grande finale we will now show that this is impossible. Let $j$ be such that $x_j=0$ and pick $i$ such that $|x_i|\leq |{x}_k|$ and $\scal{a_i,a_j}\neq 0$. That this can be done follows from the basic fact that $m+1$ non-zero vectors in $\R^m$ can not be mutually orthogonal (suppose for the moment that no $a_i$ is identically 0). Since $x_j=0$, it is no restriction to assume that $\scal{a_i,a_j}> 0$, which we do for simplicity. Consider again $x(t)=x+t e_i- te_j$. The previous analysis can now be repeated without modification, to conclude that \eqref{po0} holds whether $i>k$ or not. But in this case \eqref{po0} has a strictly negative value, which contradicts that $x$ is in $G$ to begin with. In the case when one $a_i=0$, we have $\|a_i-a_j\|_2\leq 1$ for any other $a_j$, which also yields a contradiction in \eqref{po0}.

We can finally conclude that any minimizer of $\ksir$ in $[-R,R]^n$ is in $P_k$ and thus also a minimizer of $\ksi$. Since $R$ could be arbitrarily large, the conclusion holds also in $\R^n$. The set of global minimizers of $\ksir$ is thus closed and non-empty. However, the remaining argument becomes easier if we keep $R$ fixed where it is for a while longer.

Now consider a path-connected component $H$ of the set of global minimizers in $[-R,R]^n$. Repeating the entire above argument, we see that $P_k\cap H\neq\emptyset$. Assume now that it contains points that are not in $P_k$. Since $\sum_{j=l+1}^n |\tilde x_j|$ is a continuous function on $H$ which is 0 at $P_k$, there are points in $H$ with arbitrarily small quotient $(\sum_{j=l+1}^n|\tilde x_j|)/{|\tilde x_1|}$. Recall that we have ruled out the case $0\in H$ early on in the proof, so the quotient is a continuous function on $H$. Let $I$ be a level set of this function. We repeat the construction of sets $I_n\supset I_{n-1}\supset \ldots I_{k+1}$ precisely as we did with $G$. Pick a concrete $x\in I_{k+1}$, and as before it is no restriction to assume that $x=|\tilde x|$. As before we see that it is impossible to have $ x_n=0$, and as before we can pick $i,j$ such that $\scal{a_i,a_j}\geq 0$ where $i,j>k$. We define $x(t)$ via \eqref{function} and establish as before that the \eqref{po0} must hold, whereby we get that $x(t)\in I_{k+1}$ for small values of $t$, and this contradicts how the sets $I_1,\ldots, I_k$ were chosen.

By this we get that all global minimizers of $\ksir$ in $[-R,R]^n$ must lie in $P_k$, and since $R$ can be arbitrarily large, the proof about global minimizers is complete.

Finally if we assume that $A$ is strictly $k$-feasible and that $x$ is a local minimizer, then we can always find $i,j$ such that \eqref{po0} holds, which is a contradiction since  $-4+2\|a_i-a_j\|_2^2<0$ in this case.

\end{proof}

%If $\scal{a_i,a_j}\neq 0$ for all $i,j$ or if $\|A\|_{\infty,col}\leq 1$ then the above proof is easily modified to show that any local minimizer of $\ksir$ lies in $P_k$ and is a local minimizer also for $\ksi$. We omit the details.

\subsection{On the uniqueness of sparse stationary points}

We now give a condition, similar to \eqref{e4} in Section \ref{erai}, to ensure that a sparse stationary point is unique, in the sense that other stationary points must have higher cardinality.

\begin{theorem}\label{thm:statpoint:vecfix}
Let $x'$ be a stationary point of $\ksir$ with cardinality $k$, let $z'$ be given by \eqref{y}, and assume that
\begin{equation}\label{e4fix}|\tilde z'_{k+1}|<(1-2\delta_{2k}^-)|\tilde z'_{k}|.\end{equation}
If $x''$ is another stationary point of $\ksir$ then $\card(x'') > k$.
\end{theorem}

Again, we allow $\delta_{2k}^-<0$ in the above theorem, in which case the condition on $z$ is automatically satisfied. We begin with a lemma. Recall $\G$ given by \eqref{gdef}, i.e.~$\frac{1}{2}\Q_2(\iota_{P_k})(x)+\frac{1}{2}\fro{x}$ in the present case. We need an expression for $\partial\G(x)$ for $x\in P_k$.

\begin{lemma}\label{sun}
If $x\in P_k$ then $z\in\partial\G(x)$ if and only if $\tilde z_j=\tilde x_j$ for $j=1,\ldots,k$ and $\tilde z_j\in |\tilde x_k|\D $ for $j>k$.
\end{lemma}
\begin{proof}
Since $\Q_2(\iota_{P_k})+\fro{x}$ is the l.s.c. convex envelope of $\iota_{P_k}+\fro{x}$, we have that $\G(x)=\frac{1}{2}\Q_2(\iota_{P_k})+\frac{1}{2}\fro{x}$ is the double Fenchel conjugate of $\frac{1}{2}\iota_{P_k}+\frac{1}{2}\fro{x}$. The Fenchel conjugate of the latter is easily computed to $$\G^*(y)=\frac{1}{2}\sum_{j=1}^k |\tilde y_j|^2.$$ By the well-known identity $z\in\partial \G(x)\Leftrightarrow x\in\partial \G^*(z)$ (see e.g. Proposition 16.9 in \cite{bauschke2017convex}) we have $z\in\partial\G(x)$ if and only if \begin{equation}\label{t6}z=\argmax_z \re\scal{x,z}-\frac{1}{2}\sum_{j=1}^k |\tilde z_j|^2.\end{equation}
By standard results on reordering of sequences (see e.g.~Ch.~1 in \cite{simon2005trace}), this implies that the reordering of $z$ to $\tilde z$ can be chosen identical to that of $x$, which implies that $\scal{x,z}=\scal{\tilde x,\tilde z}$. Combined with $\tilde{x}_j=0$ for $j>k$, we see that \eqref{t6} turns into \begin{equation}\label{t7}z=\frac{1}{2}\argmax_z-\sum_{j=1}^k |\tilde x_j-\tilde z_j|^2.\end{equation} The lemma now easily follows.
\end{proof}

\begin{proof}[Proof of Theorem \ref{thm:statpoint:vecfix}.]
If $\card (x'')\leq k$ we clearly have $x''-x'\in P_{2k}$ and both $z'$ and $z''$ have the structure stipulated in Lemma \ref{sun}. Let $I'=\supp x'$ and $I''=\supp x''$. Then $\re\scal{z''-z',x''-x'}$ can be written
\begin{equation}
\re\left(\sum_{\footnotesize
\begin{array}{c}
i \in I' \\
i \in I''\end{array}}
|x_i''-x_i'|^2 +
\sum_{\footnotesize
\begin{array}{c}
i \in I' \\
i \notin I''\end{array}}
(x_i'-z_i'')\overline{x_i'} +
\sum_{\footnotesize
\begin{array}{c}
i \notin I' \\
i \in I''\end{array}}
(x_i''-z_i')\overline{x_i''}\right).
\label{eq:sum1}
\end{equation}
As before we want to reach a contradiction to Proposition \ref{thm:statpoint}, i.e.~we want to prove $\re\scal{z''-z',x''-x'}>\delta_{2k}^-\|x''-x'\|_2^2$. Note that
\begin{equation}\label{gr2}
\|x''-x'\|_2^2=\sum_{\footnotesize
\begin{array}{c}
i \in I' \\
i \in I''\end{array}}
|x_i''-x_i'|^2 +
\sum_{\footnotesize
\begin{array}{c}
i \in I' \\
i \notin I''\end{array}}
|x_i'|^2 +
\sum_{\footnotesize
\begin{array}{c}
i \notin I' \\
i \in I''\end{array}}
|x_{i}''|^{2},
\end{equation}
that the first term in \eqref{eq:sum1} and \eqref{gr2} are the same, and that $\delta_{2k}^-<1$. Since the second and third sums have the same number of terms it suffices to show that
\begin{equation}
\re (x_i'-z_i'')\overline{x_i'} + (x_j''-z_j')\overline{x_j''} > \delta_{2k}^-(|x_i'|^2 + |x_j''|^{ 2}),
\label{eq:twoterms}
\end{equation}
for any pair $i\in I'$, $i\notin I''$ and $j \notin I'$, $j \in I''$. This in turn will follow upon showing that
$$|z_i''| |x_i'| + |z_j'| |x_j''| < (1-\delta_{2k}^-)(|x_i'|^2 + |x_j''|^{ 2}).$$
By Lemma \ref{sun} it is easy to see that $|z_i''|\leq |z_j''|=|x_j''|$ and by assumption we also have $|z_j'|< (1-2\delta_{2k}^-)| z'_{i}|=(1-2\delta_{2k}^-)| x'_{i}|$. Thus \begin{equation*}\begin{split}|z_i''| |x_i'| + |z_j'| |x_j''|  <  |x_j''||x_i'| + (1-2\delta_{2k}^-)| x'_{i}| |x_j''| & = 2(1-\delta_{2k}^-)| x'_{i}| |x_j''| \\ & \leq (1-\delta_{2k}^-)(|x_i'|^2 + |x_j''|^{ 2}),\end{split}\end{equation*}
as desired.
\end{proof}

\iffalse
For later use in [..], we record that we have shown the following result. \begin{corollary}\label{corbor1}
Let $z'$ satisfy $2z'\in\partial \G(x')$ and
\begin{equation*}|\tilde z'_{k+1}|<(2\lambda^2-1)|\tilde z'_{k}|.\end{equation*}
If $2z''\in\partial \G(x'')$, then $\re\scal{z''-z',x''-x'}>(1-\lambda^2)\|x''-x'\|_2^2$.
\end{corollary}
\fi

\subsection{Conditions on global minimality.}
The statements in this section are actually a bit stronger than the corresponding ones in Section  \ref{erai1}.

\begin{theorem}\label{thm:globalpoint2f}
Let $A$ be $k$-feasible and let $x'\in P_k$ be a stationary point of $\ksir$. Let $z'$ be given by \eqref{y} and assume that \eqref{e4fix} applies. Then $x'$ is a unique global minimizer of $\ksi$ and $\ksir$. If $A$ is strictly $k$-feasible, then there are no other local minimizers either.
\end{theorem}
\begin{proof}
By Theorem \ref{celok6} there exists $x''\in P_k$ which is a global minimizer for both $\ksi$ and $\ksir$. If $x'\neq x''$ this would contradict Theorem \ref{thm:statpoint:vecfix}. If in addition $A$ is strictly $k$-feasible, then Theorem \ref{celok6} says that any local minimizer is a stationary point in $P_k$, which is impossible by Theorem \ref{thm:statpoint:vecfix}.
\end{proof}

\subsection{Noisy data.}
We now assume that $b$ is of the form $Ax_0+\ep$ where $\ep$ is noise and $x_0$ is sparse. More precisely we set $S=\supp x_0$ where we assume that $\#S=k$.
Let $A_S$ denote the matrix obtained from $A$ by setting columns outside of $S$ to $0$. By minor modifications of the proof of Proposition \ref{p1} we obtain.

\begin{proposition}\label{p1f}
Let $A$ satisfy $\|A\|_{\infty,col}\leq 1$. If $|x_{0,j}|>\para{1+\frac{1}{\sqrt{1-\delta_k^-}}}\|\ep\|_2$ for all $j\in S$ then the oracle solution $x'=x_S$ is a strict local minimizer of $\ksir$ with $\supp (x')=\supp (x_0)$. This also satisfies $|x'_j|>\|\epsilon\|_2$, $j\in S$, $\|Ax'-b\|_2\leq \|\epsilon\|_2$ and $$\|x'-x_0\|_2\leq \frac{\|\ep\|_2}{\sqrt{1-\delta_k^-}}.$$
\end{proposition}

\begin{proof}
We assume for simplicity that we work over $\R$, and as in Proposition \ref{p1} we let $x'$ be the oracle solution. All estimates of Proposition \ref{p1} go through with minor modifications, for example \eqref{sofg} is replaced by \begin{equation}\label{hy}|x_{j}'|\geq |x_{0,j}|-|\de_j|>|x_{0,j}|-\frac{\|\ep\|_2}{\sqrt{1-\delta_k^-}},\quad j\in S\end{equation} which shows that $\supp (x')=\supp (x_0)$ as well as $|x'_j|>\|\epsilon\|_2$ for $j\in S$.
The only real difference is the proof that $x'$ is a local minimizer of $\ksir$, so we consider $\ksir(x'+v)$ where as usual we can assume that $x'=|\tilde x'|$. Since $x'$ solves the least squares problem posed initially, the vector $A_S^*(Ax'-b)=A_S^*(A_Sx'-b)$ must be 0, and so \begin{equation*}\ksir(x'+v)=\Q_2(\iota_{P_k})(x'+v)+2\sum_{j=k+1}^n v_j\scal{a_j,Ax'-b} +\|Av\|_2^2+\ksir(x').\end{equation*} Let $k_1$ be such that $x_{k+1-k_1}=x_k$ but $x_{k-k_1}>x_k$, and note that $k_*$ will depend on $v$ but will always satisfy $k_*\leq k_1$. With this in mind $\Q_2(\iota_{P_k})(x'+v)$ becomes \[\begin{split} & \frac{1}{k_*}\left(k_*x_k+\sum_{j=k-k_*+1}^k v_j+\sum_{j=k+1}^n|v_j|\right)^2-\sum_{j=k-k_*+1}^k(x_k+v_j)^2-\sum_{j=k+1}^n v_j^2 \\ & = k_* x_k ^2 + 2 x_k \sum_{j=k-k_*+1}^k v_j + 2 x_k \sum_{j=k+1}^n |v_j| - k_* x_k ^2 -  2 x_k \sum_{j=k-k_*+1}^k v_j + P(v)  \end{split}\] where \(P(v) \) is a quadratic function in \(v\) only. Therefore after the cancellations we are left with
$2x_k\sum_{j=k+1}^n|v_j|$ plus quadratic terms in $v$.
Returning to the expression for $\ksir(x'+v)$ and collecting all quadratic contributions from $v$ in a term $q(v)$, we see that $\ksir(x'+v)-\ksi(x')$ equals
\begin{equation*}2x_k\left(\sum_{j=k+1}^n|v_j|\right)+2\left(\sum_{j=k+1}^n v_j\scal{a_j,Ax'-b}\right) +q(v).\end{equation*}
Since $|\scal{a_j,Ax'-b}|\leq\|\epsilon\|_2$ and $x_k>\|\epsilon\|_2$, it is easy to see that there exist some constant $\rho>0$ such that \begin{equation*}2x_k\left(\sum_{j=k+1}^n|v_j|\right)+2\left(\sum_{j=k+1}^n v_j\scal{a_j,Ax'-b}\right)\geq\rho\sqrt{\sum_{j=k+1}^nv_j^2}\end{equation*} for \(v\) in a neighborhood of $0$. As in the proof of Proposition \ref{p1} we conclude that we must have $\sum_{j=k+1}^nv_j^2=0$ in order for $\ksir(x'+v)\leq \ksir(x')$ to be possible. However, for $v$ with $\supp v\subset S,$ $\Q_2(\iota_{P_k})(x'+v)=0$ and so $$\ksir(x'+v)=\|A(x'+v)-b\|_2^2\geq \|Ax'-b\|_2^2=\ksir(x'),$$ and the proof is complete.

\end{proof}

To go from saying that $x'$ is a strict local minimizer to saying unique global minimizer is now a short step.

\begin{theorem}\label{cor:dogadgetf}
Let $A$ be $k$-feasible and $\delta_{2k}^->1/{2}$. If $$|x_{0,j}|>\para{\frac{1}{1-2\delta_{2k}^-}+\frac{1}{\sqrt{1-\delta_k^-}}}\|\ep\|_2,\quad j\in S$$ then the oracle solution $x'$ in the above proposition is a global minimum of $\ksi$ and $\ksir$. Moreover, if $A$ is strictly $k$-feasible then $\ksir$ has no other local minimizers.
\end{theorem}
\begin{proof}
Proposition \ref{p1f} clearly applies and  ensures that $x'$ is a local minimizer. We now check that \eqref{e4fix} applies for $z'$ given by \eqref{y}, i.e. we want to check that $|\tilde z'_{k+1}|<(1-2\delta_{2k}^-)|\tilde z'_k|$. Note that $|\tilde z'_{k+1}|\leq\|\ep\|_2$ by the same estimate as \eqref{o0}. Moreover, since $z'\in\partial \G(x')$, Lemma \ref{sun} implies that it suffices to show that $\|\ep\|_2<(1-2\delta_{2k}^-)|\tilde x'_k|$, which by \eqref{hy} follows if
$$\|\ep\|_2<(1-2\delta_{2k}^-)\para{|\tilde x_{0,k}|-\frac{\|\ep\|_2}{\sqrt{1-\delta_k^-}}}$$ which easily is seen to be equivalent with the condition in the statement. The desired conclusions now follow by Theorem \ref{thm:globalpoint2f}.
\end{proof}
